# Supplementary material for: Atomistic study of the long-lived quantum coherences in the Fenna-Matthews-Olson complex
Source: arXiv:1104.2943 source file (2011-12-09)
Supplement: Supplementary file 1 [file BiophysJ-Supplementary.pdf]

# Supporting Material

## I. HIERARCHY EQUATION OF MOTION METHOD AND COMPARISON TO MD-METHOD

In this section, we will briefly describe the HEOM approach. The interested reader can find the details in previously published work [1, 2].

The total quantum Hamiltonian can be partitioned in its system and bath components as

$$H = H_S + H_B + H_{SB}, \tag{1}$$

where the bath is modeled by a series of harmonic oscillators as $H_B = \sum_{m=1}^{7} \sum_{i=1}^{N_{mB}} T_{mi} + \frac{1}{2} m_{mi} \omega_{mi}^2 q_{mi}^2$ which represent the phonon modes of the environment ($N_{mB}$ modes coupled to each of the seven sites $m$) and the modes of different sites are assumed to be uncorrelated. In the interaction picture, one can write the evolution of the system density matrix by tracing over the bath degrees of freedom and assuming factorized initial conditions as

$$\tilde{\rho}_S(t) = \tilde{U}_S(t)\, \tilde{\rho}_S(0) \tag{2}$$

where

$$\tilde{U}_S(t) = \left\langle \mathcal{T}_{\leftarrow} \exp\left( -\frac{i}{\hbar} \int_0^t dt_1 \tilde{\mathcal{L}}^{SB}(t_1) \right) \right\rangle_B \tag{3}$$

and $\tilde{\mathcal{L}}^{SB}(t)$ is the system-bath Liouvillian. Carrying out the cumulant expansion and using Wick's theorem for the Gaussian fluctuations one can obtain the following equation of motion of the system density operator

$$\rho_S(t) = -\frac{i}{\hbar} \mathcal{L}^S \rho(t) + \sum_{m=1}^{7} \Phi_m \sigma^{\boldsymbol{\delta}_m}(t) \tag{4}$$

where $\boldsymbol{\delta}_m = (\delta_{1m}, \delta_{2m}, ..., \delta_{mm}, .., \delta_{7m}) = (0, 0, ..., 1, ..., 0)$, $\Phi_m = i\,|m\rangle\langle m|^{\times}$ and the auxiliary operators $\sigma(t)$ in the interaction picture are defined as

$$\tilde{\sigma}^{(n_1,n_2,...,n_7)}(t) = \mathcal{T}_{\leftarrow} \prod_{m=1}^{7} \left[ \int_0^t dt_1 e^{-\gamma_m (t-t_1)} \tilde{\Theta}_j(t_1) \right]^{n_m} exp\left[ \int_0^t dt_1 \tilde{W}_m(t_1) \right] \tilde{\rho}_S(0)\,. \tag{5}$$

Such auxiliary operators evolve in time as

$$\frac{\partial}{\partial t} \sigma^{(n_1,n_2,...,n_7)}(t) = -\frac{i}{\hbar}\mathcal{L}^S - \sum_m n_m \gamma_m \sigma^{(n_1,n_2,...,n_7)}(t) \tag{6}$$

$$+ \sum_m \Phi_m \sigma^{(n_1,...,n_{m+1},..,n_7)}(t) + \sum_m n_m \Theta_m \sigma^{(n_1,...,n_{m-1},...,n_7)}. \tag{7}$$

This hierarchy theoretically continues to infinity but generally one can truncate it after a finite number of auxiliary operators and reach convergence.

The HEOM equations are not time local and therefore the phonon modes of the bath for each site are influenced by the electronic states of the chromophore at that site. Hence, the dynamics also explicitly includes site-dependent reorganization processes of the bath. Such effects are not explicitly included in the MD-method because the energy trajectories

are obtained from the one-way interaction of the bath with the system. Furthermore, the MD bath is a ground state equilibrium bath while the HEOM includes a non-equilibrium excited state bath. Finally, the MD method does not explicitly contain a memory kernel which could take into account non-Markovian effects. Nonetheless, it appears that the MD-method can reproduce correctly the experimentally observed dynamic energy transfer time scales. One could therefore argue that the reorganization processes are not dominant for the FMO complex dynamics. This argument is further supported by the fact that the MD dynamics are very similar to the HSR model, described in the next section, which does not explicitly include any reorganization energy.

## II. HAKEN-STROBL-REINECKER MODEL

The Haken-Strobl-Reinecker model is a markovian model in which the environment is described by classical stochastic variables [3, 4]. We assume that thermal fluctuations of the environment couple to the chromophores by the electron-phonon Hamiltonian:

$$H_{\mathrm{SB}}(t) = \sum_m q_m(t)|m\rangle\langle m|, \tag{8}$$

where the $q_m(t)$ describe stochastic bath fluctuations. Here, we consider only diagonal fluctuations which are typically larger than fluctuations of the inter-molecular couplings [5]. The random variables $q_m(t)$ are taken to be unbiased Gaussian fluctuations, with $\langle q_m(t)\rangle = 0$ and a two-point correlation function:

$$\langle q_m(t)q_n(0)\rangle = \delta_{mn}\delta(t)\gamma_m, \tag{9}$$

where $\gamma_m$ is the site-dependent dephasing rate. In our simulations, such rates are taken directly from the MD results as in Eq (8) of Section IIIB. We assume that fluctuations at different sites are uncorrelated and that the phonon correlation time is small compared to the system timescales. With these assumptions, one obtains the Haken-Strobl equation for the density operator in the Schrödinger picture as [3, 4]:

$$\dot{\rho}(t) = -\frac{i}{\hbar}[H_{\mathrm{S}}, \rho(t)] + L_\phi(\rho(t)), \tag{10}$$

where the pure-dephasing Lindblad operator is given by:

$$L_\phi(\rho(t)) = \sum_m \gamma_m[A_m\rho(t)A_m^\dagger - \frac{1}{2}A_mA_m^\dagger\rho(t) - \frac{1}{2}\rho(t)A_mA_m^\dagger]. \tag{11}$$

with the generators $A_m = |m\rangle\langle m|$ and pure dephasing rates $\gamma_m$. This Lindblad equation leads to exponential decay of all coherences in the density operator and to an equal distribution of populations in the inifinite time limit.

---

## SUPPORTING REFERENCES

[1] Ishizaki, A. and Fleming, G. R. Unified treatment of quantum coherent and incoherent hopping dynamics in electronic energy transfer: reduced hierarchy equation approach. *J. Chem. Phys.* **130**, 234111 (2009).

[2] Zhu, J., Kais, S., Rebentrost, P., and Aspuru-Guzik, A. Modified scaled hierarchical equation of motion approach for the study of quantum coherence in photosynthetic complexes. *J. Phys. Chem. B* **115**, 1531–7 (2011).

[3] Haken, H. and Reinecker, P. The coupled coherent and incoherent motion of excitons and its influence on the line shape of optical absorption. *Z. Phys.* **249**, 253-268 (1972).

[4] Haken, H. and Strobl, G. An exactly solvable model for coherent and incoherent exciton motion. *Z. Phys.* **262**, 135–148 (1973).

[5] Adolphs, J. and Renger, T. How proteins trigger excitation energy transfer in the FMO complex of green sulfur bacteria. *Biophys. J.* **91**, 2778–97 (2006).

## FIGURE LEGENDS

### Figure 1

Simulated linear dichroism and circular dichroism spectra at 300K.

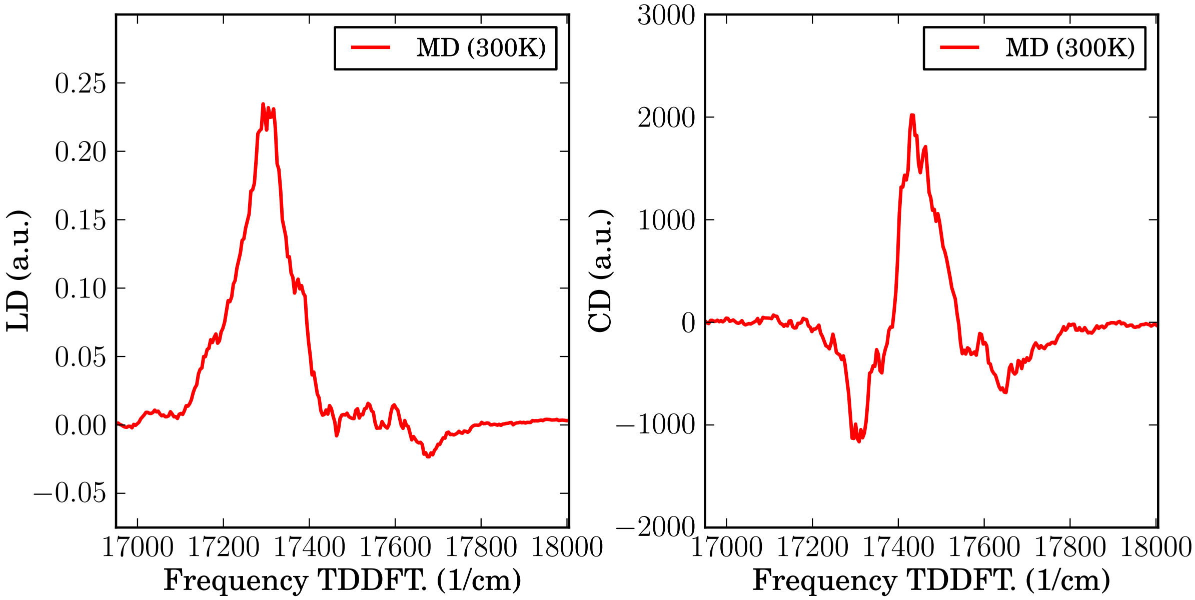

MD (300K)
LD (a.u.)
0.25
0.20
0.15
0.10
0.05
0.00
−0.05
17000 17200 17400 17600 17800 18000
Frequency TDDFT. (1/cm)
MD (300K)
CD (a.u.)
3000
2000
1000
0
−1000
−2000
17000 17200 17400 17600 17800 18000
Frequency TDDFT. (1/cm)


FIG. 1.
